# Supplementary material for: Geometrically frustrated, mechanical metamaterial membranes: Large-scale stress accumulation and size-selective assembly
Source: arXiv:2406.16790 ancillary file (2024-06-24)
Supplement: Supplementary file 1 [file Wang_2024_SI.pdf]

# Geometrically frustrated, mechanical metamaterial membranes: Large-scale stress accumulation and size-selective assembly Supplementary Information

Michael Wang, Sourav Roy, Christian Santangelo, Gregory Grason

June 24, 2024

## 1 Rigid subunits and relaxation

To simulate the relaxation of an assembly of frustrated, square-twist cuboids, we model our subunits as a rigid collection of attractive and repulsive sites. Consider a subunit positioned at  $(0,0,0)$  and oriented such that its normal points along the  $z$ -axis and its four vertical edges lie along the  $x$  and  $y$  axes. The positions of the attractive sites on its north  $(+y)$ , south  $(-y)$ , east  $(+x)$ , and west  $(-x)$  edges are given respectively by

$$\text{North: } \begin{cases} 0\hat{x} + \left(\frac{a}{2} \pm \frac{t}{2} \tan \frac{\alpha_y}{2}\right) \hat{y} \pm \frac{t}{2} \hat{z}, & \text{Vertical} \\ \pm \frac{w}{2} \hat{x} + \frac{a}{2} \hat{y} + 0\hat{z}, & \text{Horizontal} \end{cases} \quad (\text{S1})$$

$$\text{South: } \begin{cases} 0\hat{x} - \left(\frac{a}{2} \pm \frac{t}{2} \tan \frac{\alpha_y}{2}\right) \hat{y} \pm \frac{t}{2} \hat{z}, & \text{Vertical} \\ \pm \frac{w}{2} \hat{x} - \frac{a}{2} \hat{y} + 0\hat{z}, & \text{Horizontal} \end{cases} \quad (\text{S2})$$

$$\text{East: } \begin{cases} \left(\frac{a}{2} \pm \frac{t}{2} \tan \frac{\alpha_x}{2}\right) \hat{x} + 0\hat{y} \pm \frac{t}{2} \hat{z}, & \text{Vertical} \\ \frac{a}{2} \hat{x} \pm \frac{w}{2} \hat{y} + 0\hat{z}, & \text{Horizontal} \end{cases} \quad (\text{S3})$$

$$\text{West: } \begin{cases} -\left(\frac{a}{2} \pm \frac{t}{2} \tan \frac{\alpha_x}{2}\right) \hat{x} + 0\hat{y} \pm \frac{t}{2} \hat{z}, & \text{Vertical} \\ -\frac{a}{2} \hat{x} \pm \frac{w}{2} \hat{y} + 0\hat{z}, & \text{Horizontal} \end{cases} \quad (\text{S4})$$

where  $\alpha_x, \alpha_y$  are the dihedral angles. These attractive sites translate and rotate rigidly with the subunit. These subunits have specific interactions where only north sites bind to south sites (red, orange, yellow) and east sites bind to west sites (blue, blue-green, green), as shown in Figure S1. When bound, the corresponding attractive sites interact through idealized springs with stiffnesses  $k$  and zero rest length given by the potential  $U(\mathbf{r}) = \frac{1}{2}k\mathbf{r}^2$ .

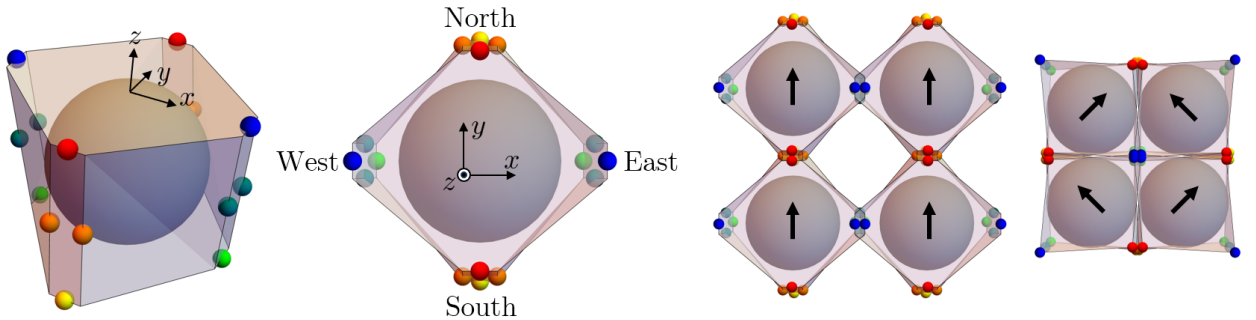

Figure S1: Subunit design and location of attractive and repulsive sites. Specific binding occurs between like colors. Central gray particle provides volume exclusion so that subunit cannot overlap when twisting (right).

### 1.1 Initialization of trumpets

To form an initial cylinder with a circumference of  $M$  subunits and a length of  $N$  subunit, we start by arranging the subunits in an  $M \times N$  square lattice in the  $xy$ -plane with centers located at  $ma\hat{x} + na\hat{y} + 0\hat{z}$  for  $0 \leq m \leq M-1$  and  $0 \leq n \leq N-1$ . We then roll this sheet into a cylinder. Note that due to the counter-rotation of neighboring subunits,  $M$  must be even so that each subunit can rotate opposite of its neighbors. The radius of a cylinder with  $M$  subunits along its hoop is  $R = a \left(\tan \frac{\pi}{M}\right)^{-1}$ . The center of subunit  $(m, n)$  undergoes the following translation

$$ma\hat{x} + na\hat{y} + 0\hat{z} \longrightarrow R \cos\left(\frac{2\pi m}{M}\right) \hat{x} + na\hat{y} + R \sin\left(\frac{2\pi m}{M}\right) \hat{z}, \quad (\text{S5})$$

and is rotated about the  $-\hat{y}$  axis by an angle  $\frac{2\pi m}{M} + \frac{\pi}{2}$ .

### 1.2 Excluded volume

To capture the effect of excluded volume so that subunits cannot overlap with each other, we add a single repulsive particle to the center of the cube whose size is roughly equal to that of the cuboids, as shown by the gray central particle in Figure S1. To be more precise, we model the excluded volume of the cuboids using a Weeks-Chandler-Andersen (WCA) potential

$$U_{\text{WCA}}(\mathbf{r}) = \begin{cases} 4\epsilon \left[ \left(\frac{\sigma}{r}\right)^{12} - \left(\frac{\sigma}{r}\right)^6 \right] + \epsilon, & r \leq 2^{1/6}\sigma \\ 0, & r > 2^{1/6}\sigma \end{cases}. \quad (\text{S6})$$

We choose  $\sigma = a/\sqrt{2}$  so that cuboids at most twist by an angle  $\approx \pi/4$  until their faces come into contact (Figure S1, right).

### 1.3 Relaxation

The assemblies are relaxed by computing the forces and torques on each subunit at each step and then translating and rotating by integrating the overdamped equations of motion, effectively performing energy minimization. In other words, the position  $\mathbf{r}_i$  of subunit  $i$  is updated via

$$\mathbf{r}_i(t + \delta t) = \mathbf{r}_i(t) + \delta t \mathbf{f}_{\text{tot}}, \quad (\text{S7})$$

where  $\mathbf{f}_{\text{tot}} = \sum_{\text{sites}} \mathbf{f}_{\text{site}}$  is the total force acting on all the attractive and repulsive sites and  $\delta t$  is the step size. For the rotation of the subunit, we compute the total torque  $\boldsymbol{\tau}_{\text{tot}} = \sum_{\text{sites}} \mathbf{r}_{\text{site}} \times \mathbf{f}_{\text{site}}$  and rotate the subunit about the unit vector  $\mathbf{r}_{\text{tot}}/|\mathbf{r}_{\text{tot}}|$  by an angle  $\delta t |\mathbf{r}_{\text{tot}}|$ . Note that for these rotations, we treat the subunit as effectively spherical such that the moment of inertial (or friction) is the identity matrix. For the purposes of determining the ground-state, this choice is sufficient.

## 2 Föppl-van Kármán theory of frustrated dilational metamembrane

The continuum elasticity framework for a mono-mode mechanical material [1], allows us to propose an energy density of the following form

$$\mathcal{W} = \int dA \left\{ \frac{1}{2} \left[ E^{ijkl} (\epsilon_{ij} - \Omega G_{ij}) (\epsilon_{kl} - \Omega G_{kl}) \right] + \frac{B}{2} (\boldsymbol{\kappa} - \bar{\boldsymbol{\kappa}})^2 + W_0(\Omega) + \frac{C_{\nabla}}{2} \bar{g}^{ij} \partial_i \Omega \partial_j \Omega \right\} \quad (\text{S8})$$

where,  $\Omega$  is the scalar field capturing the soft mode in the system and  $G_{ij}$  corresponds to the mechanism of the system. In the case of a dilational 2D metamaterial, the mechanism couples to the trace of in-plane strain.  $E^{ijkl}$  refers to the elasticity tensor for a linear, isotropic and uniform 2D material and hence characterised by the two Lamé parameters  $\lambda$  and  $\mu$ .  $B$  is the bending modulus for a 2D sheet. For the rest of the analysis, the generally non-linear function  $W_0$  is specialized to a quadratic function of  $\Omega$ . Under generic deformations, the system pays energy cost in displacement along the stiff mode,

due to gradients in the soft modes (Nambu-Goldstone modes of the broken symmetry), and the soft modes themselves.

$$\mathcal{W}(\boldsymbol{\varepsilon}, \boldsymbol{\kappa}, \Omega) = \int dA \left\{ \frac{1}{2} [(\lambda + \mu)(\varepsilon_{\text{dil}} - \Omega)^2 + 2\mu\varepsilon_{\text{dev}}^2] + \frac{B}{2} (\boldsymbol{\kappa} - \bar{\boldsymbol{\kappa}})^2 + \frac{C_{\text{mech}}}{2} |\Omega|^2 + \frac{C_{\nabla}}{2} |\nabla\Omega|^2 \right\}. \quad (\text{S9})$$

where, for a dilational metamembrane, mechanism matrix is  $\mathbf{G} = \mathbb{1}_{2 \times 2}$ ,  $\varepsilon_{\text{dil}} = \text{Tr}\boldsymbol{\varepsilon}$  is the dilational strain and  $\boldsymbol{\varepsilon}_{\text{dev}} = \boldsymbol{\varepsilon} - \mathbb{1}\varepsilon_{\text{dil}}$  is the deviatoric strain.

For purposes of analytical computation, we specialize into adopting an axisymmetric (cylindrical) geometry with a preferred curvature  $\kappa_{\parallel}$  in the axial direction (along  $\hat{\mathbf{z}}$ ). The undeformed cylinder of radius  $R$  deforms via an axially symmetric deflection  $\zeta(z)$  and in-plane displacement  $u_z(z)$ . In the cylindrical coordinate system, the 3D coordinates of the deformed sheet is the following  $\tilde{\mathbf{R}} = (R + \zeta)\hat{\mathbf{r}} + (z + u_z)\hat{\mathbf{z}}$ . In the Föppl-Von Kármán limit, the total elastic energy is

$$\mathcal{W} = \int dA \left\{ \frac{1}{2} Y \left( \frac{\zeta(z)}{R} - \Omega(z) \right)^2 + \frac{C_{\text{mech}}}{2} \Omega(z)^2 + \frac{C_{\nabla}}{2} |\nabla\Omega(z)|^2 + \frac{1}{2} B (\zeta''(z) - \kappa_{\parallel})^2 \right\}, \quad (\text{S10})$$

where  $Y = \frac{4\mu(\lambda+\mu)}{\lambda+2\mu}$  is the 2D Young's modulus. The modulus  $B$  is the bending modulus of the meta-material sheet.

With free boundary conditions, varying Eq. (S10), we arrive at the following coupled equations of motion

$$\left( \ell_{\text{flat}}(\text{stiff}) \right)^4 \frac{d^4}{dz^4} \tilde{\zeta} + (\tilde{\zeta} - \Omega) = 0 \quad (\text{S11})$$

$$\ell_{\text{mech}}^2 \Delta\Omega - \frac{C_{\text{mech}}}{Y} \Omega + (\tilde{\zeta} - \Omega) = 0 \quad (\text{S12})$$

where,  $\tilde{\zeta} = \zeta/R$  is the fractional deflection and  $\ell_{\text{flat}}(\text{stiff}) = (B/Y)^{1/4} R^{1/2}$  and  $\ell_{\text{mech}} = \sqrt{C_{\nabla}/Y}$  are two emergent length scales. Due to the soft modes the enhanced flattening length scale becomes  $\ell_{\text{flat}}(\text{floppy}) = (B/C_{\nabla})^{1/2} R$ , which demarcates the onset of flattening transition after the intermediate soft *liquid crystalline* energy accumulation zone. The linear ODEs obtained in Eq. (S11) and (S12), can be solved with the ansatz:  $a_1 \cosh r_1 z + a_2 \cosh r_2 z + a_3 \cosh r_3 z$ , for field variable  $\tilde{\zeta}$ , where  $\{r_1, r_2, r_3\}$  refer to the roots of the characteristic polynomial of the corresponding uncoupled ODE. The constants  $\{a_1, a_2, a_3\}$  can be fixed by respecting the boundary conditions  $\zeta''(z)|_{\partial} = \kappa_{\parallel}$  and  $\zeta'''(z)|_{\partial} = \Omega'(z)|_{\partial} = 0$ , thus giving an exact solution for this axisymmetric trumpet like geometry.

### 3 Continuum limit of discrete subunit model

We here derive a version of the continuum elastic theory of a frustrated trumpet with dilations starting from the discrete building blocks. Consider an  $M \times N$  sheet that is rolled up into a tube that is  $M$  subunits around the hoop. We start with a cylindrical reference state where subunit  $(m, n)$  is located at a radius  $r^{(m, n)} = \frac{a}{2} \cot \frac{\pi}{M}$ , angle  $\theta^{(m, n)} = \frac{2\pi m}{M}$ , and height  $z^{(m, n)} = na$  and whose normal is pointing radially outward. Based on observations from discrete simulations, we make several assumptions to simplify the derivation (Figure S2).

- The first assumption is that subunits with the same  $m$  (i.e. a column of subunits along  $z$ ) maintain the same angle  $\frac{2\pi m}{M}$  and only undergo radial displacements  $u_r^{(m, n)}$ .
- The second assumption is that the normals of the subunits can only tilt along the  $z$  direction by an angle  $\phi^{(m, n)}$ , and that the subunits rotate about their normals by a twist angle  $\psi^{(m, n)}$ .

We further simplify assuming asymmetry and with radial displacements and tilts that depend only on the position  $n$  along the tube i.e.  $u_r^{(m, n)} = u_r^{(n)}$  and  $\phi^{(m, n)} = \phi^{(n)}$ . Similarly, the magnitude of the twist must also be independent of  $m$  but since neighboring subunits must counter-rotate, we must have  $\psi^{(m, n)} = (-1)^{m+n} \psi^{(n)}$ . The axisymmetry allows us to derive the continuum limit by only considering the stretching of the bonds between subunits  $(m, n)$ ,  $(m, n+1)$ , and  $(m \pm 1, n)$ ,

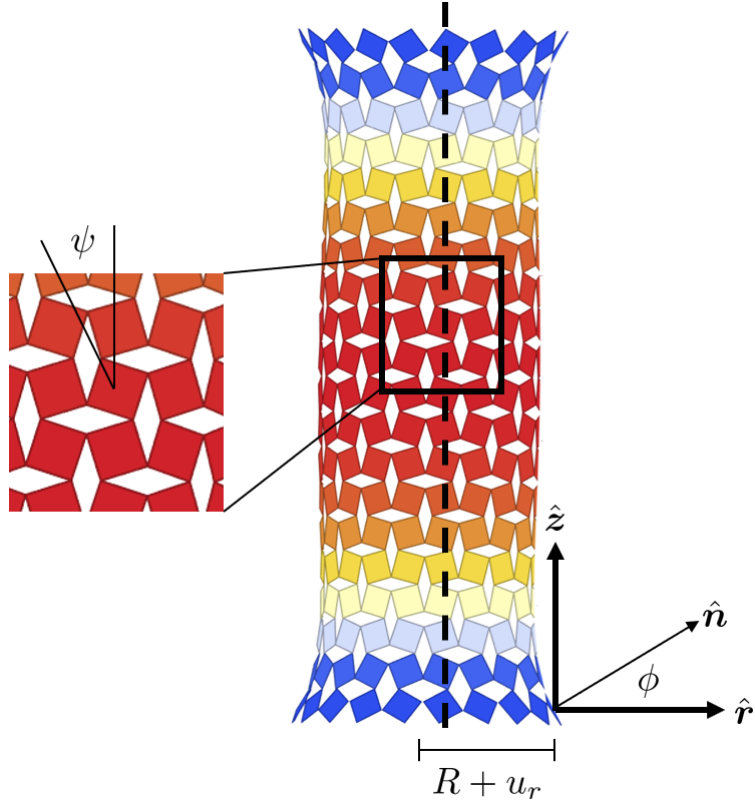

Figure S2: Approximations for describing the in-plane twist  $\psi$ , tilt  $\phi$ , and radial displacements  $u_r$  of subunits on the surface of a frustrated trumpet.

and then simply summing over  $n$  and every other  $m$  in the large  $N$  and  $M$  limits, assuming slowly varying displacement and twist. The continuum elastic theory can then be obtained by taking  $a \rightarrow 0$  while holding the curvatures  $\kappa_{\parallel} = 2 \tan \alpha_{\parallel} / a$  and  $\kappa_{\perp} = 2 \tan \alpha_{\perp} / a$  fixed and using the following approximation

$$\frac{f^{(n+1)} - f^{(n)}}{a} \approx \frac{df}{dz}, \quad (\text{S13})$$

where  $f$  is  $u_r$ ,  $\phi$ , or  $\psi$ .

The resulting continuum model for elastic energy assuming a closed trumpet with preferred diameter,  $R\kappa_{\perp} = 1$  and small twist ( $\phi \ll 1$ ),

$$\begin{aligned} \mathcal{W} = \frac{1}{L} \int_{-\frac{L}{2}}^{\frac{L}{2}} dz & \left[ \frac{1}{2} Y \left( \frac{du_r}{dz} + \phi \cos \psi \right)^2 + \frac{1}{2} Y \left( \frac{du_z}{dz} + 1 - \cos \psi \right)^2 + \frac{1}{2} B \left( \frac{d\phi}{dz} + \kappa_{\parallel} \cos \psi \right)^2 \right. \\ & \left. + \frac{1}{2} Y \left( \frac{u_r}{R} + 1 - \cos \psi \right)^2 + \frac{1}{2} B \frac{(1 - \cos \psi)^2}{R^2} + \frac{1}{2} K_{\psi} \sin^2 \psi + \frac{1}{2} K_{\nabla\psi} \left( \frac{d \sin \psi}{dz} \right)^2 \right]. \end{aligned} \quad (\text{S14})$$

Here, the moduli in terms of the discrete subunit parameters are given by  $Y = 4k$  (stretch),  $B = kt^2/2$  (bend),  $K_{\psi} = 2kw^2/a^2$  (twist), and  $K_{\nabla\psi} = ka^2$  (twist gradient). Note that the displacements  $u_z$  along the tube can be integrated out and written as  $u_z(z) = -\int_0^z dz' [1 - \cos \psi(z')]$ .

To compare to the FvK theory, we observe that the frustrated trumpets have some characteristic twist  $\psi_0$  about which there are deviations. Linearizing about that point  $\psi = \psi_0 + \delta\psi$ , leads a continuum

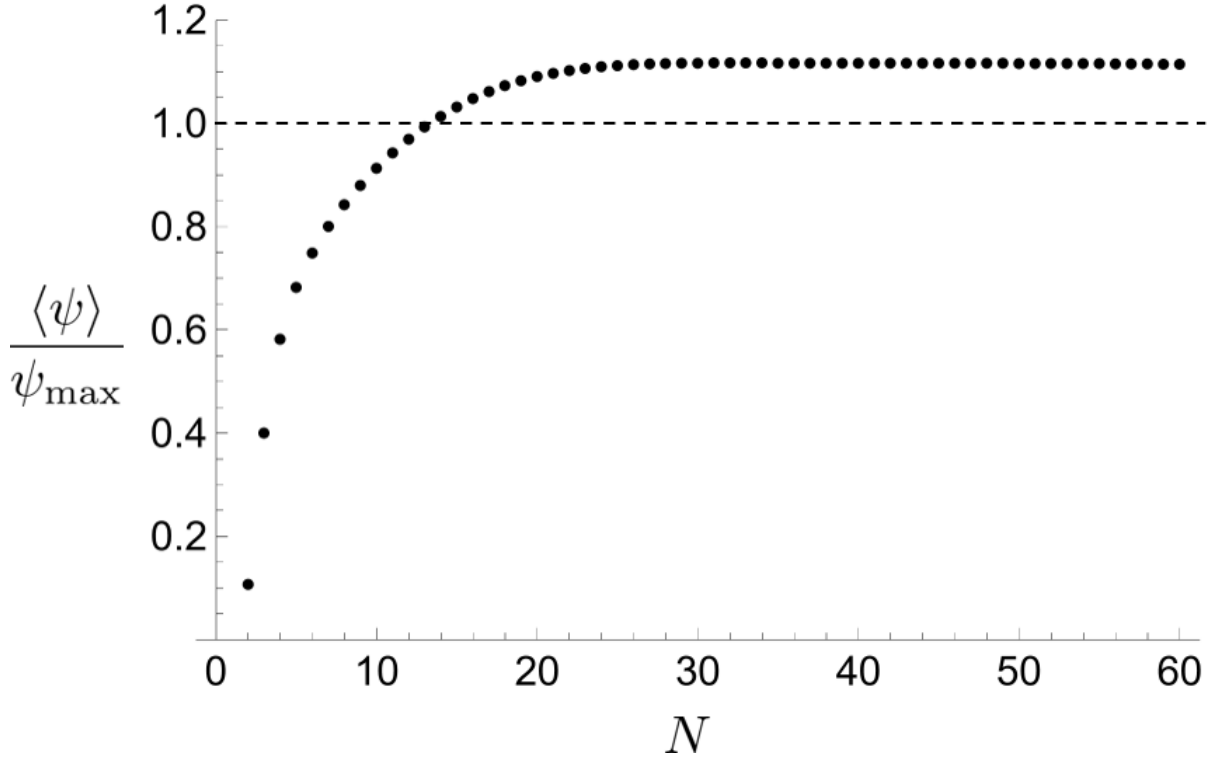

Figure S3: Average twist throughout trumpet as a function of size for  $\kappa_{\perp} = \pi/28$  and  $\kappa_{\parallel} = (3/4)\kappa_{\perp}$ . The maximum twist is  $\psi_{\max} = \pi/4$ .

energy of the form in Eq. (S10), (S14) as

$$\begin{aligned} \mathcal{W} = \frac{1}{L} \int_{-\frac{L}{2}}^{\frac{L}{2}} dz & \left[ \frac{1}{2} Y \left( \frac{du_r}{dz} + \phi \cos \psi_0 \right)^2 + \frac{1}{2} B \left( \frac{d\phi}{dz} + \kappa_{\parallel} \cos \psi_0 - \kappa_{\parallel} \sin \psi_0 \delta \psi \right)^2 \right. \\ & + \frac{1}{2} Y \left( \frac{u_r}{R} + 1 - \cos \psi_0 + \sin \psi_0 \delta \psi \right)^2 + \frac{1}{2} B \frac{(1 - \cos \psi_0 + \sin \psi_0 \delta \psi)^2}{R^2} \\ & \left. + \frac{1}{2} K_{\psi} (\sin \psi_0 + \cos \psi_0 \delta \psi)^2 + \frac{1}{2} K_{\nabla \psi} \cos^2 \psi_0 \left( \frac{d\delta \psi}{dz} \right)^2 \right] \end{aligned} \quad (\text{S15})$$

If we define  $\hat{u}_r = u_r + R(1 - \cos \psi)$ , we note the following relation between between the theories (i.e. eqs. S10 and S15)

$$\frac{1}{2} Y \left( \frac{\hat{u}_r}{R} + \sin \psi_0 \delta \psi \right)^2 \longleftrightarrow \frac{1}{2} Y \left( \frac{\zeta}{R} - \Omega \right)^2, \quad (\text{S16})$$

which determines the mechanism field to be  $\Omega = -\sin \psi_0 \delta \psi$ , and

$$C_{\nabla} = K_{\nabla \psi} \cot^2 \psi_0. \quad (\text{S17})$$

In Fig. S3, we plot the value of average twist of a floppy trumpet (for parameters studied in main text Fig. 2), showing that the characteristic twist is varies from  $0.1\psi_{\max}$  for short-trumpets up to  $1.1\psi_{\max}$  for large trumpets, where  $\psi_{\max} = \pi/4$  for a square-twist mechanism. Using the average value of  $0.6\psi_{\max}$  to estimate  $\psi_0$  over this accumulating range we estimate a ratio of  $C_{\nabla}/K_{\nabla \psi} \approx 4$  in this range. In main text. Fig. 2, we plot the continuum model for a constant for  $C_{\nabla} = 4K_{\nabla \psi}$  to account for the numerical offset between the gradient mechanism cost in the FvK theory and the continuum limit of our frustrated cuboid model. The comparison shows reasonable agreement, notwithstanding, the crude nature of this parameter estimation and the considerable variation of  $\psi_0$  values with length exhibited by the discrete metamembrane model.

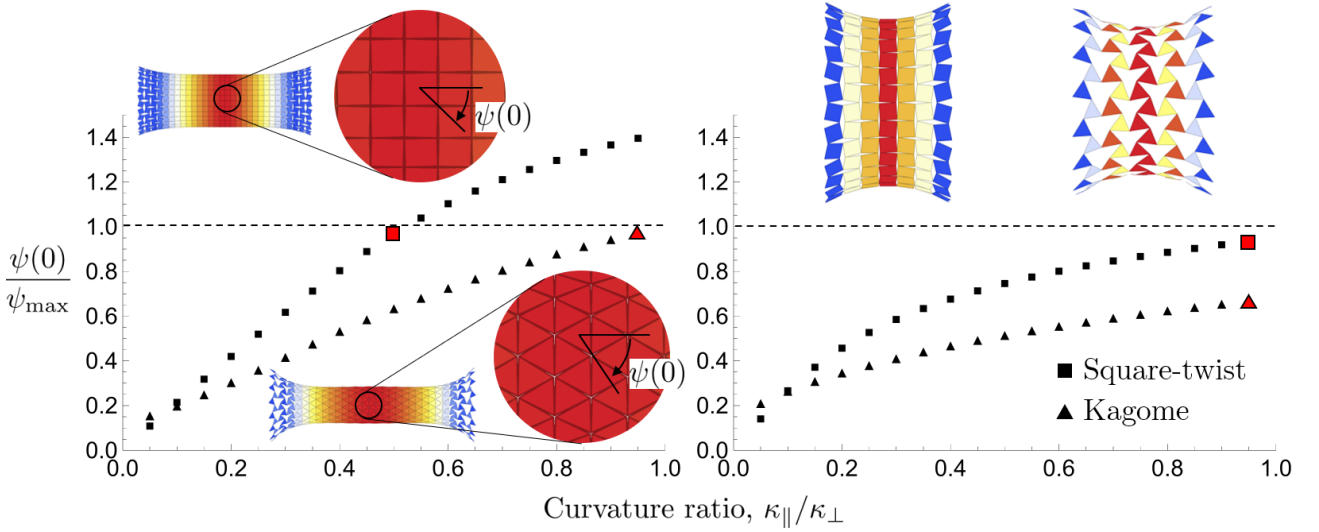

Figure S4: Amount of twist or dilation  $\psi(0)$  at the center of trumpets as functions of the curvature ratio  $\kappa_{||}/\kappa_{\perp}$ . The maximum twist angles  $\psi_{\max}$  due to excluded volume for square-twist and kagome mechanisms are  $\pi/4$  and  $\pi/3$ , respectively. **Left:** Square-twist trumpets with 30 subunits along hoop ( $\perp$ ) and 30 subunits along tube ( $\parallel$ ). Kagome trumpets with 30 subunits along hoop ( $\perp$ ) and 58 subunits along tube ( $\parallel$ ). **Right:** Square-twist trumpets with 30 subunits along hoop ( $\perp$ ) and 7 subunits along tube ( $\parallel$ ). Kagome trumpets with 30 subunits along hoop ( $\perp$ ) and 10 subunits along tube ( $\parallel$ )

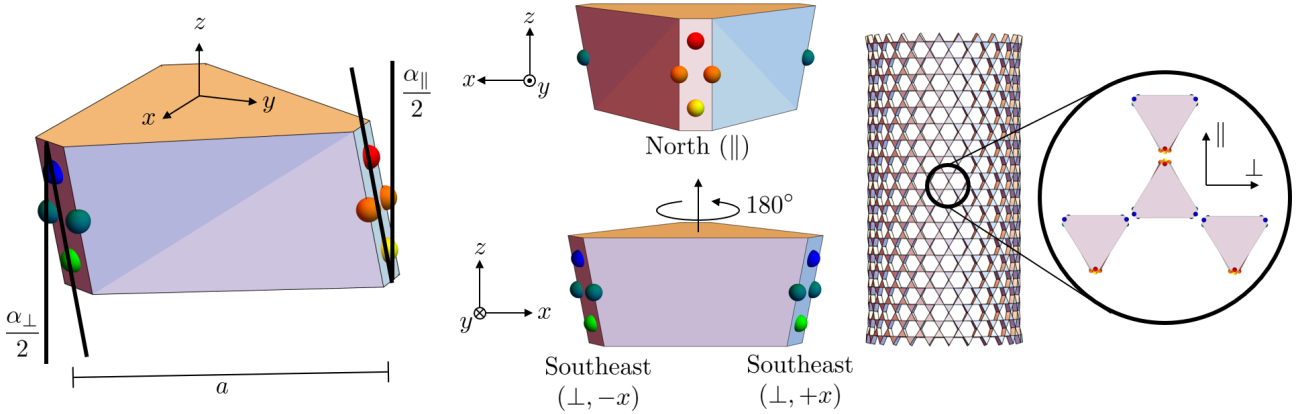

Figure S5: Subunit design for frustrated Kagome lattice of triangular prisms.

## 4 Characteristic twist vs curvature ratio

As shown in Figure S4 left, the twist angle  $\psi(0)$  at the center of the long trumpets ( $L > L_{\text{flat}}$ ) for a square-twist mechanisms exceeds the maximum  $\psi_{\max}$  allowed by excluded volume when  $\kappa_{||}/\kappa_{\perp} \gtrsim 0.5$ . For a Kagome mechanism, however, up to  $\kappa_{||}/\kappa_{\perp} \sim 1$ , the triangular subunits do not overlap. For shorter trumpets ( $L < L_{\text{flat}}$ ), shown in Figure S4 right, this twist angle decreases below the maximum.

## 5 Kagome subunits

Unlike the cuboid design where the dihedral angles  $\alpha_{\perp}$  and  $\alpha_{||}$  can easily be translated into the target curvatures, determining the dihedrals for the three corners of a triangular block is less intuitive. The dihedral angles can be determined from with a slight modification to [2]. We start by defining the following function

$$\kappa(\alpha_i, \alpha_j) = \frac{\sqrt{3}(\sin \alpha_i + \sin \alpha_j)(\cos \alpha_i + \cos \alpha_j + \cos \alpha_i \cos \alpha_j - 2 \sin \alpha_i \sin \alpha_j - 3)}{a[4 \cos \alpha_i + \cos \alpha_j - 8 \cos(\alpha_i - \alpha_j) + 3 \cos 2\alpha_i + 3 \cos \alpha_j - 6]} \quad (\text{S18})$$

Given the dihedral angles  $\alpha_{\parallel}$  and  $\alpha_{\perp}$ , the hoop and tube curvatures  $\kappa_{\perp}$  and  $\kappa_{\parallel}$  are defined as

$$\kappa_{\perp} = \kappa(\alpha_{\perp}, \alpha_{\perp}) \quad (\text{S19a})$$

$$\kappa_{\parallel} = \frac{4\kappa(\alpha_{\parallel}, \alpha_{\perp}) - \kappa_{\perp}}{3}. \quad (\text{S19b})$$

These can be used to determine the dihedral angles in terms of the target curvatures. Figure S5 shows the design of a Kagome subunit and the specific binding of warmer colors (red, orange, yellow) along the tube direction ( $\parallel$ ) and cooler colors (blue, blue-green, green) along the hoop direction ( $\perp$ ). For a subunit centered at  $(0, 0, 0)$  oriented such that its normal is in the  $\hat{\mathbf{z}}$  direction and its  $\parallel$  direction sites point to the  $\hat{\mathbf{y}}$  direction, the attractive sites along its north ( $\parallel$ ), southeast ( $\perp, +x$ ), and southwest edges ( $\perp, -x$ ) are located at

$$\text{North } (\parallel): \begin{cases} 0\hat{\mathbf{x}} + \left(\frac{a\sqrt{3}}{3} \pm \frac{t}{2} \tan \frac{\alpha_{\parallel}}{2}\right) \hat{\mathbf{y}} \pm \frac{t}{2} \hat{\mathbf{z}}, & \text{Vertical} \\ \pm \frac{w}{2} \hat{\mathbf{x}} + \frac{a\sqrt{3}}{3} \hat{\mathbf{y}} + 0\hat{\mathbf{z}}, & \text{Horizontal} \end{cases} \quad (\text{S20})$$

$$\text{Southeast } (\perp, +x): \begin{cases} \left(\frac{a}{2} \pm \frac{t\sqrt{3}}{4} \tan \frac{\alpha_{\perp}}{2}\right) \hat{\mathbf{x}} - \left(\frac{a\sqrt{3}}{6} \pm \frac{t}{4} \tan \frac{\alpha_{\perp}}{2}\right) \hat{\mathbf{y}} + \pm \frac{t}{2} \hat{\mathbf{z}}, & \text{Vertical} \\ \left(\frac{a}{2} \pm \frac{w}{4}\right) \hat{\mathbf{x}} - \left(\frac{a\sqrt{3}}{6} \mp \frac{w\sqrt{3}}{4}\right) \hat{\mathbf{y}} + 0\hat{\mathbf{z}}, & \text{Horizontal} \end{cases} \quad (\text{S21})$$

$$\text{Southwest } (\perp, -x): \begin{cases} -\left(\frac{a}{2} \pm \frac{t\sqrt{3}}{4} \tan \frac{\alpha_{\perp}}{2}\right) \hat{\mathbf{x}} - \left(\frac{a\sqrt{3}}{6} \pm \frac{t}{4} \tan \frac{\alpha_{\perp}}{2}\right) \hat{\mathbf{y}} + \pm \frac{t}{2} \hat{\mathbf{z}}, & \text{Vertical} \\ -\left(\frac{a}{2} \pm \frac{w}{4}\right) \hat{\mathbf{x}} - \left(\frac{a\sqrt{3}}{6} \mp \frac{w\sqrt{3}}{4}\right) \hat{\mathbf{y}} + 0\hat{\mathbf{z}}, & \text{Horizontal} \end{cases} \quad (\text{S22})$$

## References

- [1] S. Roy and C. D. Santangelo. Curvature screening in draped mechanical metamaterial sheets. *Soft Matter*, 19:8150–8156, 2023.
- [2] B. Tyukodi, F. Mohajerani, D. M. Hall, G. M. Grason, and M. F. Hagan. Thermodynamic size control in curvature-frustrated tubules: Self-limitation with open boundaries. *ACS Nano*, 16:9077, 2022.
